# Supplementary material for: Wrinkling of Random and Regular Semiflexible Polymer Networks
Source: arXiv:1406.1302 source file (2014-06-05)
Supplement: Supplementary file 1 [file supplemental_material.pdf]

# Supplementary Information for "Wrinkling of random and regular semiflexible polymer networks"

Pascal Müller and Jan Kierfeld
*Physics Department, TU Dortmund University, 44221 Dortmund, Germany*

In this Appendix, we present details of the simulation model of the crosslinked semiflexible polymer network and a summary of the wrinkling theory based on continuum linear elasticity theory used to analyze our simulation results. We also present details on how wrinkling affects the crossover from bending to stretching dominated deformation of the network.

PACS numbers: 46.32.+x, 87.16.Ka, 87.16.dm, 46.70.De

## SIMULATION

In this Appendix, we present details of the simulation model of the crosslinked semiflexible polymer network.

### Network preparation

We analyze and compare two types of semiflexible polymer networks: (i) random and (ii) regular networks. For both types of networks, the initial condition is planar.

(i) Random networks are prepared using a "mikado model" [1, 2]. In a rectangular simulation box of size $L_x \times L_y$ in the $x$-$y$-plane, straight rods of length $L$ are added at random positions and random angles. Intersections between rods are identified as crosslinks. The resulting mean distance between neighboring crosslinks is $l_c$, and rods are added until a given density $\eta = L/l_c$ is reached. In order to allow bending deformation, the resulting segments between crosslinks are split into two by adding a midpoint. Dangling ends are removed as they can relax freely and do not contribute to the total elastic energy.

(ii) Regular triangular networks are prepared by placing infinitely long rods equidistantly and at angles $\varphi = 0, \pi/3, 2\pi/3$ with respect to the $x$-direction. Again we identify intersections as crosslinks, and add midpoints to the resulting segments of equal length $l_c^\triangle$.

For both types of networks, we apply periodic boundary conditions in $x$-direction and fixed boundary conditions in $y$-direction, i.e., intersection points with the boundary are treated as fixed crosslinks.

As a result, the network configuration is defined by a set of points (crosslinks and midpoints) with two main properties: (a) the position in three-dimensional space and (b) a list of connections to neighboring points. In order to calculate the stretching energy, the initial segment lengths $l_{ij,0}$ between pairs $ij$ of neighboring points are also stored. Crosslinks are connected to 2-4 other points in random networks and to 6 other points in regular triangular networks; midpoints always have two neighboring points.

### Semiflexible polymer network model

We use a simulation model very similar to the model presented in Ref. [1]. The stretching energy $E^{(s)} = (\mu/2)\int ds (u'(s))^2$ is applied to each pair $ij$ of neighboring points connected by a rod segment, the bending energy $E^{(b)} = (\kappa/2)\int ds(\phi'(s))^2$ is applied to each triple $ijk$ of neighboring points connected by segments along the *same* rod.

The stretching energy of a segment of length $l_{ij}$ with $u'(s) \approx (l_{ij} - l_{ij,0})/l_{ij,0}$ is

$$E_{ij}^{(s)} = \frac{\mu}{2}\frac{(l_{ij} - l_{ij,0})^2}{l_{ij,0}} \ . \quad (1)$$

The bending energy of a triple $ijk$ of neighboring points with the two neighboring segments forming an angle $\phi_{ijk}$ is

$$E_{ijk}^{(b)} = \kappa \frac{1-\cos\phi_{ijk}}{l_{ij} + l_{jk}} \ . \quad (2)$$

Here we used $(\phi'(s))^2 \approx 2(1-\cos\phi_{ijk})/(l_{ij}+l_{jk})^2$. These definitions can be applied both to planar and wrinkled networks.

### Energy Minimization

For energy minimization, we used a conjugate gradient method which minimizes the total stretching and bending energy of the network. The degrees of freedom are the positions of crosslinks and midpoints.

For the gradient method, we calculate stretching and bending forces on each crosslink and midpoint. The stretching force $\mathbf{F}_{i,ij}^{(s)}$ onto point $i$ (with position $\mathbf{r}_i$, i.e., $l_{ij} = |\mathbf{r}_i - \mathbf{r}_j|$ and with $\mathbf{l}_{ij} \equiv \mathbf{r}_i - \mathbf{r}_j$) from a link $ij$ is

$$F_{i,ij}^{(s)} = -\mu \frac{\mathbf{l}_{ij}}{l_{ij}} \frac{l_{ij} - l_{ij,0}}{l_{ij,0}} \ .$$

A point $i$ is subject to bending forces as an endpoint of a triple $ijk$ or as a midpoint of a triple $jik$. The bending

force $\mathbf{F}^{(b)}_{i,ijk}$ acting upon an endpoint $i$ of a triple $ijk$ is

$$\mathbf{F}^{(b)}_{i,ijk} = \kappa \frac{\mathbf{l}_{ij}}{l_{ij}} \left[ \frac{1-\cos\phi_{ijk}}{(l_{ij}+l_{jk})^2} - \frac{1}{l_{ij}+l_{jk}} \left( \frac{\cos\phi_{ijk}}{l_{ij}} + \frac{1}{l_{jk}} \right) \right],$$

whereas the force on a midpoint is given by

$$\mathbf{F}^{(b)}_{i,jik} = \kappa \frac{1-\cos\phi_{ijk}}{(l_{ij}+l_{ik})^2} \left( \frac{\mathbf{l}_{ij}}{l_{ij}} + \frac{\mathbf{l}_{ik}}{l_{ik}} \right) - \kappa \frac{1}{l_{ij}+l_{ik}} \left[ \cos\phi_{ijk} \left( \frac{\mathbf{l}_{ij}}{l_{ij}^2} + \frac{\mathbf{l}_{ik}}{l_{ik}^2} \right) + \frac{\mathbf{l}_{ij}+\mathbf{l}_{ik}}{l_{ij} l_{ik}} \right].$$

All stretching and bending forces on a point $i$ have to be added up to get the total force $\mathbf{F}_i$, which is used in the conjugate gradient algorithm.

In a planar network, there are no resulting forces in the $z$-direction, and the network remains planar without a perturbation.

### Simulation parameters

We use square systems of sizes $L_x/L = L_y/L = 1.5$ for random networks. We investigated random network densities $\eta = L/l_c = 32...54$ and regular network densities $\eta' = L_x/l_c^\Delta = 20...50$. The random network densities are chosen well above the percolation threshold and sufficiently high to avoid network configurations with low density regions, where wrinkling patterns are not well-defined.

Filament elasticity is characterized by the length scale $l_b \equiv \sqrt{\kappa/\mu}$, for which we consider a parameter range $l_b/L = 1.4 \cdot 10^{-4}...2.5 \cdot 10^{-3}$.

### Network deformation and preconditioning

Simulations are performed by increasing the shear angle $\gamma$ of the simulation box by increments ranging from $10^{-7}$ to $10^{-2}$ depending on elastic properties of the network and the range of shear angles that we want to study. In each step $n$, the boundaries of the simulation box are fixed at a new angle $\gamma_n = \gamma_{n-1} + \delta\gamma$, and an affine deformation with $\delta x(y) = y \sin\gamma$ is applied to all points. This includes the intersection points with the $y$-boundaries at $y = 0$ and $y = L_y$, which are fixed at their new positions after the affine deformation. Then, the minimization routine is used to let the network relax into its new equilibrium configuration with respect to the positions of the remaining interior crosslinks and midpoints.

Since the forces have no $z$-component in a strictly planar network, it remains planar under shear. However, the planar unwrinkled state becomes an unstable (or metastable) minimum above a critical shear angle, $\gamma > \gamma_c$, and we can induce wrinkling by applying small perturbations. To probe the stability of the planar state, we randomly perturb crosslinks and midpoints in $z$-direction with a random amplitude $\delta z(x, y)$. We increase the random amplitude until the resulting increase in energy $\delta E$ reaches a certain value relative to the total energy of the network before perturbation - usually between 1 and 10%.

We also use non-random perturbations in order to calculate the wrinkling threshold $\gamma_c$. In this case, we apply displacements according to the wrinkling pattern $z(x, y)$ that is expected from elasticity theory at the onset of wrinkling, see eq. (15) below.

For some simulations of random networks, we use a "preconditioning" procedure: we first calculate a wrinkle pattern for a regular network with similar elastic properties, measure the displacement pattern $z(x, y)$ (eventually interpolating from the lattice points in the $xy$-plane), and apply the *same* displacement pattern to the random network. This is only done once before the start of the simulation.

### Wrinkle detection

To determine wrinkles and measure their wavelength $\lambda$, we calculate all intersection points of rod segments with the $xy$-plane. For wrinkled configurations, these points are arranged in a pattern of parallel lines. The distance between these lines equals $\lambda/2$.

In order to determine the wrinkle amplitude, we calculate the square sum of the $z$-components of all $N$ points in the network, $\sum_{i=1}^N z_i^2$. Assuming an approximately uniform area per point, we compare this to the integral $\frac{N}{L_x L_y} \int dxdy \, (z(x, y))^2$ over a continuous wrinkling pattern $z(x, y)$ as it is expected from elasticity theory, see eq. (15) below. We use the measured wavelength $\lambda$ and solve for the amplitude of this pattern. This procedure can be applied to both regular and random networks.

### Wrinkling threshold

For regular networks, we can use the relation $A^2 \propto (\gamma - \gamma_c)$, see (22) below, to obtain the threshold shear $\gamma_c$ for the onset of wrinkling in our simulations. We extrapolate the square of the wrinkling amplitude $A^2$ as a function of shear angle linearly (for $\gamma > \gamma_c$), and the zero of this line is $\gamma_c$. To determine $\gamma_c$, we impose wrinkling perturbations following the pattern (15) given below with the longest admissible wavelength $\lambda = \lambda_1 = L_x/\sqrt{2}$ ($n = 1$).

For random networks, we find that the amplitude exhibits discrete jumps instead of approaching zero continuously as $A^2 \propto (\gamma - \gamma_c)$. In this case, we identify $\gamma_c$ as the first shear angle exhibiting a non-zero wrinkling am-

plitude $A > 0$ upon imposing a wrinkling perturbation (15) with $n = 1$.

## CONTINUUM ELASTICITY THEORY OF WRINKLING UNDER SHEAR

In this Appendix, we summarize the continuum linear elastic theory of wrinkling of an elastic membrane under an applied shear strain $\gamma$, to which we compare our findings for regular and random semiflexible polymer networks. This elastic theory can be found in similar form in Refs. [3] or Ref. [4].

### Elastic moduli

The in-plane deformations of planar two-dimensional elastic membranes are characterized by a 2D Young modulus $Y$ or a compression modulus $K$, a shear modulus $G$, and a Poisson ration $\nu$. For isotropic elasticity, we have two independent elastic constants and the additional relations $G = Y/2(1+\nu)$ and $K = Y/2(1-\nu)$.

For a regular triangular network of semiflexible polymers with stretching elasticity $E^{(s)} = (\mu/2)\int ds(u'(s))^2$ and a lattice constant $l_c^\triangle$, we can calculate the elastic constants explicitly [5]:

$$G = \frac{\sqrt{3}}{4}\frac{\mu}{l_c^\triangle}\ , \quad Y = \frac{8}{3}G\ , \quad K = 2G\ , \quad \nu = \frac{1}{3} \qquad (3)$$

Out-of-plane bending deformations are characterized by a bending modulus $B$. For thin plates from a 3D isotropic material, the bending modulus is related to the 2D moduli and the plate thickness $t$ by $B = Yt^2/12(1-\nu^2)$. For a triangular network of semiflexible polymers with bending elasticity $E^{(b)} = (\kappa/2)\int ds(\phi'(s))^2$ and a lattice constant $l_c^\triangle$, the bending modulus is given by

$$B = \frac{3\sqrt{3}}{4}\frac{\kappa}{l_c^\triangle} = 3G\frac{\kappa}{\mu} = 3Gl_b^2 \qquad (4)$$

with $l_b \equiv \sqrt{\kappa/\mu}$.

### Strains, stresses, and energies

For a general deformation $\mathbf{r}(x,y) = \mathbf{r}_0(x,y) + u_1(x,y)\mathbf{e_x} + u_2(x,y)\mathbf{e_y} + z(x,y)\mathbf{e_z}$ of an elastic membrane with respect to an undeformed reference state $\mathbf{r}_0(x,y)$, length changes $dr^2 - dr_0^2 = \sum_{ij} u_{ij}dx_idx_j$ are described by a 2D strain tensor

$$u_{ij} \equiv \begin{pmatrix} \varepsilon_x & \gamma_{xy} \\ \gamma_{xy} & \varepsilon_y \end{pmatrix}, \qquad (5)$$

and a corresponding stress tensor

$$\sigma_{ij} \equiv \begin{pmatrix} \sigma_x & \tau_{xy} \\ \tau_{xy} & \sigma_y \end{pmatrix} = \begin{pmatrix} \frac{Y}{1-\nu^2}(\varepsilon_x + \nu\varepsilon_y) & 2G\gamma_{xy} \\ 2G\gamma_{xy} & \frac{Y}{1-\nu^2}(\varepsilon_y + \nu\varepsilon_x) \end{pmatrix}. \qquad (6)$$

The elastic energy density is given by

$$\begin{aligned} e_{2D} &= \frac{1}{2}\sigma_{ij}u_{ij} = Gu_{ik}^2 + \frac{1}{2}(K-G)u_{ll}^2 \\ &= \frac{1}{2}G\Delta\varepsilon^2 + 2K\bar{\varepsilon}^2 + 2G\gamma_{xy}^2 \end{aligned} \qquad (7)$$

with $\Delta\varepsilon \equiv \varepsilon_x - \varepsilon_y$ and $\bar{\varepsilon} \equiv \frac{1}{2}(\varepsilon_x + \varepsilon_y)$.

We apply a uniform shear by an angle $\gamma$ with boundary conditions $u_x(x, L_y) - u_x(x,0) = (\tan\gamma)L_y$ and $u_y(x,L_y) = u_y(x,0) = 0$ at $y = L_y$ and $y = 0$ and periodic boundary conditions in $x$-direction. For a strictly *planar* deformation in the absence of wrinkling, the resulting in-plane strain and stress tensors are *homogeneous*

$$u_{ij,pl} = \begin{pmatrix} 0 & \gamma/2 \\ \gamma/2 & 0 \end{pmatrix},\ \sigma_{ij,pl} = \begin{pmatrix} 0 & G\gamma \\ G\gamma & 0 \end{pmatrix}, \qquad (8)$$

and the elastic energy density is

$$e_{2D,pl} = \frac{1}{2}G\gamma^2. \qquad (9)$$

Wrinkling gives rise to an additional out-of-plane displacement $z(x,y)$. For small deflections, the second fundamental form $\kappa_{ij}$ of the membrane describing its curvatures is given by

$$\kappa_{ij} \approx \frac{\partial^2 z}{\partial x_i \partial x_j} + \mathcal{O}(z^2), \qquad (10)$$

and the additional in-plane strains caused by the displacement $z(x,y)$ are

$$u_{ij} = \begin{pmatrix} \varepsilon_{x,pl} + \frac{1}{2}\kappa_{11}^2 & \gamma_{xy,pl} + \frac{\partial z}{\partial x}\frac{\partial z}{\partial y} \\ \gamma_{xy,pl} + \frac{\partial z}{\partial x}\frac{\partial z}{\partial y} & \varepsilon_{y,pl} + \frac{1}{2}\kappa_{22}^2 \end{pmatrix} + \mathcal{O}(z^4) \qquad (11)$$

The total elastic energy density $e = e_{2D} + e_B$ is the sum of the in-plane elastic energy (7) and the bending energy

$$e_B = \frac{1}{2}B\left[\kappa_{11}^2 + \kappa_{22}^2 + 2\nu\kappa_{11}\kappa_{22} + 2(1-\nu)\kappa_{12}^2\right], \qquad (12)$$

see, for example, Ref. [3].

### Force equilibrium

The equilibrium configuration of the membrane is obtained by the conditions of force equilibrium, which are

$$\begin{aligned} \sum_i \partial_i\sigma_{ij} &= 0\ , \\ B\left[\frac{\partial^4 z}{\partial x^4} + \frac{\partial^4 z}{\partial y^4} + 2\frac{\partial^4 z}{\partial x^2\partial y^2}\right] &= \sum_{ij}\sigma_{ij}\kappa_{ij} \end{aligned} \qquad (13)$$

for small out-of-plane displacements $z(x, y)$.

These equations are the first variation of the total energy $e_{2D} + e_B$ as given by (7) and (12) with respect to the fields $u_{ij}$ and $z(x, y)$. The first equation represents the in-plane force equilibrium, the second equation the force equilibrium perpendicular to the plane.

**Wrinkling instability (near threshold)**

In order to calculate the wrinkling pattern $u_{ij}$ and $z(x, y)$ for a given shear angle $\gamma$ exactly, we have to solve the equations (13) with the correct boundary conditions. An alternative approximate procedure is to choose a suitable ansatz $z(x, y)$ for the out-of-plane wrinkling pattern, assume homogeneous in-plane strains as in (8), and minimize the total elastic energy $e_{2D} + e_B$ with respect to the parameters of the ansatz $z(x, y)$ [3].

For a planar shear deformation (8), the strain tensor is diagonal in a $\xi$-$\eta$ coordinate system rotated by $\pi/4$, i.e., $\xi \equiv (x + y)/\sqrt{2}$, $\eta \equiv (y - x)/\sqrt{2}$ with

$$u_{\xi\eta} \equiv \begin{pmatrix} \varepsilon_\xi & \gamma_{\xi\eta} \\ \gamma_{\xi\eta} & \varepsilon_\eta \end{pmatrix} = \begin{pmatrix} \gamma/2 & 0 \\ 0 & -\gamma/2 \end{pmatrix}. \tag{14}$$

The principal strain axes of the deformation are $e_\xi = (1, 1)/\sqrt{2}$ and $e_\eta = (-1, 1)/\sqrt{2}$ with pure stretching in $\xi$-direction and pure compression in $\eta$-direction. Therefore, wrinkles are expected to appear perpendicular to the $\eta$-direction of compression and along the $\xi$-direction. This motivates the ansatz

$$z(x, y) = A \sin\left(\pi \frac{y}{L_y}\right) \sin\left(2\pi \frac{y - x}{\sqrt{2}\lambda}\right) \tag{15}$$

for the wrinkling pattern with amplitude $A$ and wrinkle wavelength $\lambda$. This ansatz satisfies the boundary conditions $u_y(x, L_y) = u_y(x, 0) = 0$ at $y = L_y$ and $y = 0$. The periodic boundary conditions in $x$-direction limit the wrinkle wavelength to a set of *discrete* values

$$\lambda_n = \frac{1}{\sqrt{2}} \frac{L_x}{n} \quad (n = 1, 2, ...). \tag{16}$$

There is a maximal wavelength $\lambda_1 = L_x/\sqrt{2}$, which is admitted by the system size and the boundary conditions.

Close to the critical angle $\gamma \approx \gamma_c$, we can expand the total elastic energy $e_{2D} + e_B$ in powers of the amplitude $A$. Because of the $A \to -A$ symmetry, only even terms occur in this expansion.

The resulting in-plane and bending elastic energy densities are

$$e_{2D,wr} = \frac{1}{2} G\gamma^2 - \frac{\pi^2}{2} G\gamma \frac{A^2}{\lambda^2} + \mathcal{O}(A^4) \ , \tag{17}$$

$$e_{B,wr} = \frac{1}{2} B A^2 4\pi^4 \left[\frac{1}{\lambda^4} + \frac{1}{\lambda^2 L_y^2} + \frac{1}{16 L_y^4}\right] \ , \tag{18}$$

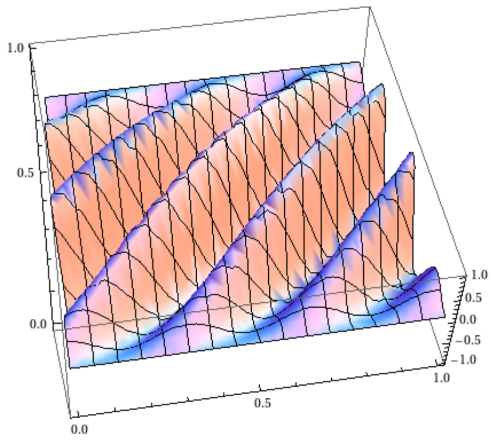

FIG. 1: Wrinkle pattern (15) for $n = 2$, i.e., $\lambda = L_x/2\sqrt{2}$.

where we replaced oscillating functions by their spatial averages over the area. The second term in (17) favors wrinkling, which relieves compressive stress in $\eta$-direction. The first term in $e_{2D,wr}$ is identical to the strictly planar elastic energy. If the energy difference $\Delta e$ between wrinkled and unwrinkled state is negative, $\Delta e = e_{2D,wr} + e_{B,wr} - e_{2D,pl} < 0$, wrinkling is energetically favorable and the planar state becomes unstable with respect to the formation of wrinkles with $A \neq 0$. This is the case when the coefficient of the $A^2$-terms in $\Delta e$ becomes negative, i.e.

$$\gamma > 4\pi^2 \frac{B}{G} \left[\frac{1}{\lambda^2} + \frac{1}{L_y^2} + \frac{\lambda^2}{16 L_y^4}\right].$$

The smallest wrinkling angle $\gamma_c$ leading to an instability is obtained for the maximal wavelength $\lambda = \lambda_1$,

$$\begin{aligned} \gamma_c &= 4\pi^2 \frac{B}{G} \left[\frac{1}{\lambda_1^2} + \frac{1}{L_y^2} + \frac{\lambda_1^2}{16 L_y^4}\right] \\ &= 4\pi^2 \frac{B}{G} \frac{1}{L_y^2} \left[2a^2 + 1 + \frac{1}{32a^2}\right] \propto B \end{aligned} \tag{19}$$

where $a \equiv L_y/L_x$ is the aspect ratio of the membrane.

The energetically most favorable and most unstable wavelength $\lambda$ for $\gamma > \gamma_c$ (but $\gamma$ sufficiently small so that we are still near threshold) is selected by minimizing $e_{2D} + e_B$ with respect to $\lambda$. This gives

$$\lambda \approx \sqrt{8}\pi \left(\frac{B}{G}\right)^{1/2} \frac{1}{\gamma^{1/2}} \tag{20}$$

for $\gamma \gg \gamma_c$. The wavelength $\lambda_n$ closest to this value will appear as wrinkling pattern.

According to eqs. (17) and (18), the energy difference is

$$\Delta e = e_{2D,wr} + e_{B,wr} - e_{2D,pl} = -a(\gamma - \gamma_c)A^2 + bA^4 \tag{21}$$

with positive coefficients $a$ and $b$ ($a \sim G/\lambda_1^2$ and $b \sim G/\lambda_1^4$). Therefore, minimizing with respect to $A$ gives

$$A^2 \propto (\gamma - \gamma_c) \tag{22}$$

at the onset of wrinkling. Therefore, the wrinkling instability is always a *supercritical pitchfork bifurcation* analogously to standard $\phi^4$-theory with a second order phase transition (as in beam buckling). The instability happens at the *largest* wavelength $\lambda_1$ that is admissible by boundary conditions, which is also similar to buckling.

We use the relation (22) to obtain $\gamma_c$ in our simulations by linearly extrapolating $A^2$ to zero as a function of shear angle.

**Wrinkling far from threshold**

For strong shear, we will have fully developed wrinkles whose amplitude $A$ grows and whose wavelength $\lambda$ decreases with increasing $\gamma$. Expansions in $A$ are no longer a good approximation. Here, we use (i) that a wrinkled network can only support little stress perpendicular to the wrinkle direction, such that $\sigma_\xi \gg |\sigma_\eta|$. This will lead to a relation between $A$ and $\lambda$. Then, we use (ii) the force equilibrium to determine $\lambda$ (alternatively, one can minimize the total energy $e_{2D} + e_B$ with respect to $\lambda$ for given $A = A(\lambda)$, see Ref. [4]).

Far from the threshold, we start from $\sigma_\eta \approx 0$. Actually, $\sigma_\eta$ will be of the order of the critical stress of a plate of width $\lambda/2$, i.e., $\sigma_\eta \sim -\sigma_{cr} = -4\pi^2 B/\lambda^2$ [4], and we assume $\sigma_\xi \gg \sigma_{cr}$. In contrast, at the onset of wrinkling, we assumed that both stresses are approximately equal, $\sigma_\xi \approx \sigma_\eta \approx G\gamma$, with only *small* corrections of order $\mathcal{O}(A^2)$ from wrinkles. Using $\sigma_\eta = \frac{Y}{1-\nu^2}(\varepsilon_\eta + \nu\varepsilon_\xi) \approx 0$ and $\varepsilon_\xi = \frac{1}{Y}(\sigma_\xi - \nu\sigma_\eta) \approx \frac{1}{Y}\sigma_\xi$, we find in-plane strain contributions

$$\begin{aligned} \varepsilon_\eta &= -\nu\varepsilon_\xi = -\nu\frac{\gamma}{2} \ , \\ \sigma_\xi &= Y\varepsilon_\xi = Y\frac{\gamma}{2} \ . \end{aligned} \tag{23}$$

Since wrinkles essentially lead to a vanishing stress $\sigma_\eta$, these results are reminiscent of uniaxial stretching in $\xi$-direction with stress-free boundaries, where we also find the usual lateral contraction $\varepsilon_\eta = -\nu\varepsilon_\xi$.

We assume $\gamma \gg (A/L_y)^2$ such that stress and strain in $\xi$-direction are unaffected by the wrinkles:

$$\varepsilon_\xi \approx \frac{\gamma}{2} + \frac{\pi^2}{16}\frac{A^2}{L_y^2} \approx \frac{\gamma}{2} \ .$$

The compressive strain in $\eta$-direction is relieved by wrinkling. The condition $\sigma_\eta \approx 0$ only holds in the middle of the membrane ($y = L_y/2$), where

$$\varepsilon_\eta = -\frac{\gamma}{2} + \frac{1}{2}\left(\frac{\partial z}{\partial \eta}\right)^2$$

is maximal for a wrinkling pattern (15). Averaging the strain $\varepsilon_\eta$ over one wrinkle in the middle of the membrane, we find

$$\varepsilon_\eta \approx -\frac{\gamma}{2} + \pi^2\frac{A^2}{\lambda^2} \ .$$

This gives

$$\begin{aligned} -\frac{\gamma}{2} + \pi^2\frac{A^2}{\lambda^2} &= \varepsilon_\eta = -\nu\varepsilon_\xi = -\nu\frac{\gamma}{2} \\ \frac{\gamma}{2}(1-\nu) &= \pi^2\frac{A^2}{\lambda^2} \end{aligned}$$

or

$$A = \frac{1}{\sqrt{2}\pi}(\gamma(1-\nu))^{1/2}\lambda \ . \tag{24}$$

Furthermore, the force equilibrium (13) in out-of-plane direction, which also holds for larger deflection amplitudes $A$, gives

$$\begin{aligned} B\frac{\partial^4 z}{\partial \eta^4} &\approx \sigma_\xi\frac{\partial^2 z}{\partial \xi^2} \\ B(2\pi)^4\frac{A}{\lambda^4} &\approx Y\frac{\gamma}{2}\frac{\pi^2}{2}\frac{A}{L_y^2}, \end{aligned}$$

which leads to [4]

$$\lambda = (8\pi)^{1/2}\left(\frac{B}{Y\gamma}\right)^{1/4} L_y^{1/2}. \tag{25}$$

Far from threshold, we find for elastic energy density $e_{2D,wr} + e_{B,wr} \approx \sigma_\xi\varepsilon_\xi/2 \approx Y\gamma^2/8$. Therefore, linear continuum elasticity predicts for the energy ratio $E_{wr}/E_{pl}$ of wrinkled to planar networks

$$\frac{E_{wr}}{E_{pl}} = \frac{e_{2D,wr} + e_{B,wr}}{e_{2D,pl}} = \frac{Y}{4G} = \frac{1+\nu}{2} \tag{26}$$

where we used (9) and $Y = 2(1+\nu)G$.

## CROSSOVER FROM BENDING TO STRETCHING

For small linear strains, planar random networks are bending dominated for small densities and become stretching dominated for higher densities [1, 2, 7]. For a fixed density, random networks are bending dominated at low strains and stretching dominated at high strains [6]. We find that this crossover is strongly modified by the wrinkling transition.

Onck *et al.* [6] suggest that the transition between bending and stretching dominated regimes can be identified by the following parameter measuring the deviation from affine behavior:

$$\Delta A = \frac{1}{n}\sum_{k=1}^{n} |\Delta\vec{r}_k - \Delta\vec{a}_k| \,/\, |\Delta\vec{a}_k| \ . \tag{27}$$

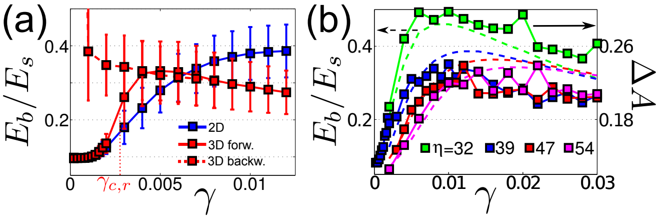


FIG. 2: (a) Ratio $E_b/E_s$ of bending to stretching energy as a function of shear angle $\gamma$ for random networks with $l_b/L = 7.9 \cdot 10^{-4}$ and $\eta = 39$. Wrinkling at $\gamma_c \simeq 0.003$ leads to an immediate crossover to stretching dominated behavior. We also observe hysteresis. (b) Ratio $E_b/E_s$ (dashed lines) and non-affinity measure $\Delta A$ (solid lines, data points) as a function of shear angle $\gamma$ for planar random networks with $l_b/L = 7.9 \cdot 10^{-4}$ and $\eta = 32$, 39, 47, 54.

Here, $n$ is the total number of points in the network, $\Delta\vec{r}_k$ are their actual displacements in a shear increment, and $\Delta\vec{a}_k$ are their displacements under an affine deformation. The transition from bending to stretching dominated behavior is expected to coincide with a maximum in $\Delta A$.

Since wrinkling is necessarily non-affine, it causes $\Delta A$ to become very large and probably even discontinuous at the wrinkling instability. Hence, $\Delta A$ is not very reliable for measuring the dominant deformation mode in wrinkled networks, and we need a different indicator. For planar networks, we find that a maximum in $\Delta A$ coincides with a maximum of the ratio of bending to stretching energy, $E_b/E_s$, see Fig. 2b. Therefore, we can use this ratio similarly to $\Delta A$ as an indicator for the transition in deformation behavior. It also has the additional advantage of being applicable in wrinkled networks without the problems we have with $\Delta A$. By comparing the same networks in planar and three-dimensional simulations, we find that wrinkling causes a transition to stretching dominated behavior at much smaller strains than in planar networks, see Fig. 2a. Because of the hysteresis at the wrinkling transition described in the main text, we can also study wrinkled networks at strains $\gamma < \gamma_{c,r}$ and find that they are always dominated by stretching. Consequently, the wrinkling transition automatically causes the network to become stretching dominated. Thus, the wrinkling instability leads to a profound modification of the network deformation behavior.


[1] D.A. Head, A.J. Levine, and F.C. MacKintosh, Phys. Rev. Lett. **91**, 108102 (2003).

[2] J. Wilhelm and E. Frey, Phys. Rev. Lett. **91**, 108103 (2003).

[3] S.P. Timoshenko and J.M. Gere, *Theory of Elastic Stability*, Tata McGraw-Hill Education (1961).

[4] W. Wong and S. Pellegrino, J. Mech. Materials Struct. **1**, 27 (2006).

[5] D. Boal, *Mechanics of the Cell*, Cambridge University Press, Cambridge (2002).

[6] P.R. Onck, T. Koeman, T. van Dillen, and E. van der Giessen, Phys. Rev. Lett. **95**, 178102 (2005).

[7] C. Heussinger and E. Frey, Phys. Rev. Lett. **96**, 017802 (2006).
